# Supplementary material for: Observation of Bloch oscillations in molecular rotation
Source: arXiv:1504.06811 ancillary file (2015-04-26)
Supplement: Supplementary file 1 [file supplementaryBO.pdf]

# Experimental observation of Bloch oscillations in molecular rotation: supplementary information

Johannes Floß,[1] Andrei Kamalov,[2] Ilya Sh. Averbukh,[1] and Philip H. Bucksbaum[2]

[1] *Department of Chemical Physics, Weizmann Institute of Science, 234 Herzl Street, Rehovot 76100, Israel*

[2] *Stanford PULSE Institute, SLAC National Accelerator Laboratory, Menlo Park, California 94025, USA*

(Dated: April 19, 2015)

In this supplementary information to the article titled "Experimental observation of Bloch oscillations in molecular rotation", we provide a formal derivation of the connection between the periodically kicked rotor and Bloch oscillations in crystalline solids.

We have developed two ways of deriving the equations of motion for the semi-classical model. One of them is applicable to small detunings from the quantum resonance and small values of the kick strength. In the second derivation, the kick strength has not to be small, however the formalism is heavy. Both of the derivations lead to the same final results. Here, we will show the former one as it is more intuitive; the second one will be left to an upcoming publication.

For the derivation we assume that the laser pulses are well approximated by delta-kicks. We also assume that the molecules can be considered as rigid rotors. The latter approximation is justified as long as the detuning from the quantum resonance is large compared to the centrifugal distortion correction of the rotational levels. In the remainder of this text we furthermore give energy in units of $2B$ (where $B$ is the rotational constant), time in units of $2\hbar/B$ and momentum in $\hbar$. The rotational revival time in these units is given as $t_{\text{rev}} = 2\pi$.

Consider any state $|\Psi\rangle$ of a linear rotor subject to a periodic train of delta-kicks with period $\tau$. The one-cycle evolution (pulse-to-pulse) of the state is described by the evolution operator $\hat{U}$:

$$|\Psi\rangle^{(n+1)} = \hat{U}|\Psi\rangle^{(n)} \tag{1}$$

Here, $|\Psi\rangle^{(n)}$ is the wave function right after the $n^{\text{th}}$ laser pulse. Each cycle consists of a free evolution, followed by a laser kick. The evolution operator is given as

$$\hat{U} = e^{iP\cos^2\theta} e^{-i\hat{J}^2\tau/2} \,. \tag{2}$$

The first term $\exp(iP\cos^2\theta)$ describes the instantaneous kick by the laser pulse, where $P$ is an effective kick strength. It is given as $P = (\Delta\alpha/4\hbar)\int E^2(t)\mathrm{d}t$, where $\Delta\alpha$ is the molecular polarisability anisotropy and $E(t)$ is the envelope of the laser electric field, and reflects the typical change of the angular momentum by a laser pulse. The second term $\exp(-i\hat{J}^2\tau/2)$ describes the free rotation between the laser pulses. Here, $\hat{J}$ is the angular momentum operator. We consider a kicking period close to the rotational revival time, $\tau = (1+\delta)t_{\text{rev}} = 2\pi(1+\delta)$, so that

$$\hat{U} = e^{iP\cos^2\theta} e^{-i\pi\hat{J}^2(1+\delta)} \,. \tag{3}$$

Using that $\exp(-i\pi\hat{J}^2)$ does not alter the rotational wave function, and that $\delta$ and $P$ are small, we can expand $\hat{U}$ as

$$\hat{U} \approx 1 - i\pi\delta\hat{J}^2 + iP\cos^2\theta \,. \tag{4}$$

We now look at the effect of $\hat{U}$ on the rotor state $|\Psi\rangle$. Therefore we expand $|\Psi\rangle$ in the rotational eigenfunctions, the spherical harmonics $|J, M\rangle$:

$$|\Psi\rangle^{(n)} = \sum_{J',M'} C^{(n)}_{J',M'}|J', M'\rangle \,. \tag{5}$$

Since the projection quantum number $M$ is conserved by the interaction, we can treat it as a parameter. Here, we only consider $M = 0$, and for simplicity omit $M$ from the notation in the following. Inserting equations (4) and (5) into equation (1) and multiplying by $\langle J|$ from the left, we get

$$C^{(n+1)}_J = C^{(n)}_J - i\pi\delta J(J+1)C^{(n)}_J + iP\sum_{J'} C^{(n)}_{J'}\langle J|\cos^2\theta|J'\rangle \,. \tag{6}$$

Using the approximation

$$\langle J|\cos^2\theta|J'\rangle \approx \begin{cases} 1/2 & \text{for} J' = J \\ 1/4 & \text{for} J' = J\pm 2 \\ 0 & \text{else} \end{cases} \tag{7}$$

as well as rearranging the terms, we get

$$i\left[C^{(n+1)}_J - C^{(n)}_J\right] = -\frac{P}{4}\left[C^{(n)}_{J+2} + C^{(n)}_{J+2}\right] + \left[\pi\delta J(J+1) - \frac{P}{2}\right]C^{(n)}_J \,. \tag{8}$$

Since the change of $C_J$ from pulse to pulse is small ($P$ and $\delta$ are small), we can approximate $C^{(n+1)}_J - C^{(n)}_J \approx \mathrm{d}C_J(n)/\mathrm{d}n$ and consider $n$ as a continuous dimensionless time. We can then recast the difference equation (8) as a differential equation,

$$i\frac{\mathrm{d}C_J(n)}{\mathrm{d}n} = -\frac{P}{4}\left[C_{J+2}(n) + C_{J+2}(n)\right] + \left[\pi\delta J(J+1) - \frac{P}{2}\right]C_J(n) \,. \tag{9}$$

Equation (9) looks like the Schrödinger equation of a particle moving in a periodic 1D lattice of $J$-sites (tight-binding model). The first term on the right hand side describes coherent transfer of the probability amplitude between the states $|J\rangle$ and $|J \pm 2\rangle$. The second term can be interpreted as resulting from an effective on-site "potential energy" of the particle. In the following, we drop the term $-P/2$, as it is simply an overall shift of the "energy". Furthermore, notice that sites of even and odd $J$ form two independent sublattices.

Let us first consider the case of the quantum resonance, i.e. pulse trains tuned exactly to the quantum resonance and $\delta = 0$. For zero detuning, the sites in the model (9) are degenerate. The solutions of equation (9) can then be given in the form of Bloch waves,

$$C_J(n) = Ae^{ikJ - i\varepsilon(k)n} \,. \tag{10}$$

Here, $k$ is the dimensionless quasi-momentum of the Bloch wave, and $\varepsilon(k)$ is the quasi-energy. Substituting equation (10) into equation (9), we obtain the dispersion relation

$$\varepsilon(k) = -\frac{P}{2}\cos(2k) \,. \tag{11}$$

The wave packet from the Bloch states (10) moves unrestrictedly through the $J$-space, reaching very high values of $J$. This is exactly what we expect for the quantum resonance, a ballistic (linear in time) and unlimited growth of $J$.

At non-zero detuning $\delta$, the degeneracy of the sites is lifted, and the individual $J$-sites are shifted in energy as if an external potential

$$V(J) = \pi\delta J(J+1) \tag{12}$$

was applied to the lattice. In the case of $\delta < 0$ (the case of our experiment), the potential $V(J)$ is an accelerating one. As $k$ increases, it eventually reaches the edge of the Brillouin zone at $k = \pi/2$, and the wave packet is reflected by Bragg reflection (remember that the "spatial" coordinate $J$ is discrete). This scenario is very similar to the one considered by Zener and Bloch, namely the problem of electrons moving in a periodic lattice and subject to an additional accelerating electric field: These electrons undergo an oscillatory motion, the Bloch oscillations. The only difference is that in the Bloch-Zener case the external potential is linear in the coordinate, whilst in our case it is quadratic. Nevertheless, this difference is not critical, and the same analysis can be applied here.

For analytical estimates, we utilised the semiclassical model that was employed by Zener and Bloch 85 years ago, and which has been widely used since then [see, e.g., Ashcroft, Mermin, Solid State Physics, (Brooks Cole; 1st Ed., 1976), chapter 12]. This model provides the following equations for the time-dependent quasi-momentum, and the mean velocity of the wave packet of Bloch states:

$$\frac{\mathrm{d}k}{\mathrm{d}n} = -\frac{\mathrm{d}V(J)}{\mathrm{d}J} \approx -2\delta J \tag{13a}$$

$$\frac{\mathrm{d}J}{\mathrm{d}n} = \frac{\mathrm{d}\epsilon(k)}{\mathrm{d}k} = P\sin(2k) \,. \tag{13b}$$

The first of these equations is just the Newton's second law (remember that $n$ is the "time"), and the second one defines the group velocity of the Bloch wave packet. The system of equations (13) can be solved in quadratures, and it indeed demonstrates an oscillatory dynamics – rotational Bloch Oscillations.
